# Supplementary material for: Bayesian Selection of sign(mu) within mSUGRA in Global Fits Including WMAP5 Results
Source: arXiv:0807.4512 source file (2008-10-22)
Supplement: Supplementary file 1 [file SM_1d.tex]

%GNUPLOT: LaTeX picture with Postscript
\begin{picture}(0,0)%
\includegraphics{SM_1d}%
\end{picture}%
\setlength{\unitlength}{0.0200bp}%
\begin{picture}(18000,10800)(0,0)%
\put(2475,7050){\makebox(0,0)[r]{\strut{} 0}}%
\put(2475,7850){\makebox(0,0)[r]{\strut{} 0.25}}%
\put(2475,8650){\makebox(0,0)[r]{\strut{} 0.5}}%
\put(2475,9450){\makebox(0,0)[r]{\strut{} 0.75}}%
\put(2475,10250){\makebox(0,0)[r]{\strut{} 1}}%
\put(3428,6500){\makebox(0,0){\strut{} 3.99}}%
\put(5462,6500){\makebox(0,0){\strut{} 4.2}}%
\put(7497,6500){\makebox(0,0){\strut{} 4.41}}%
\put(550,8650){\rotatebox{90}{\makebox(0,0){\strut{}$P/P_{max}$}}}%
\put(5462,5675){\makebox(0,0){\strut{}$m_b(m_b)^{\overline{MS}}$ (GeV)}}%
\put(11475,7050){\makebox(0,0)[r]{\strut{} 0}}%
\put(11475,7850){\makebox(0,0)[r]{\strut{} 0.25}}%
\put(11475,8650){\makebox(0,0)[r]{\strut{} 0.5}}%
\put(11475,9450){\makebox(0,0)[r]{\strut{} 0.75}}%
\put(11475,10250){\makebox(0,0)[r]{\strut{} 1}}%
\put(12428,6500){\makebox(0,0){\strut{} 165.5}}%
\put(14463,6500){\makebox(0,0){\strut{} 170.9}}%
\put(16497,6500){\makebox(0,0){\strut{} 176.3}}%
\put(9550,8650){\rotatebox{90}{\makebox(0,0){\strut{}$P/P_{max}$}}}%
\put(14462,5675){\makebox(0,0){\strut{}$m_t$ (GeV)}}%
\put(16023,9730){\makebox(0,0)[r]{\strut{}posterior}}%
\put(16023,9290){\makebox(0,0)[r]{\strut{}likelihood}}%
\put(2475,1650){\makebox(0,0)[r]{\strut{} 0}}%
\put(2475,2450){\makebox(0,0)[r]{\strut{} 0.25}}%
\put(2475,3250){\makebox(0,0)[r]{\strut{} 0.5}}%
\put(2475,4050){\makebox(0,0)[r]{\strut{} 0.75}}%
\put(2475,4850){\makebox(0,0)[r]{\strut{} 1}}%
\put(3428,1100){\makebox(0,0){\strut{} 0.1116}}%
\put(5463,1100){\makebox(0,0){\strut{} 0.1176}}%
\put(7497,1100){\makebox(0,0){\strut{} 0.1236}}%
\put(550,3250){\rotatebox{90}{\makebox(0,0){\strut{}$P/P_{max}$}}}%
\put(5462,275){\makebox(0,0){\strut{}$\alpha_s^{\overline{MS}}(M_Z)$}}%
\put(11475,1650){\makebox(0,0)[r]{\strut{} 0}}%
\put(11475,2450){\makebox(0,0)[r]{\strut{} 0.25}}%
\put(11475,3250){\makebox(0,0)[r]{\strut{} 0.5}}%
\put(11475,4050){\makebox(0,0)[r]{\strut{} 0.75}}%
\put(11475,4850){\makebox(0,0)[r]{\strut{} 1}}%
\put(12428,1100){\makebox(0,0){\strut{} 127.864}}%
\put(14462,1100){\makebox(0,0){\strut{} 127.918}}%
\put(16497,1100){\makebox(0,0){\strut{} 127.972}}%
\put(9550,3250){\rotatebox{90}{\makebox(0,0){\strut{}$P/P_{max}$}}}%
\put(14462,275){\makebox(0,0){\strut{}$1/\alpha^{\overline{MS}}$}}%
\end{picture}%
\endinput
